# Supplementary material for: Regularizing Towards Permutation Invariance in Recurrent Models
Source: arXiv:2010.13055 source file (2020-10-25)
Supplement: Supplementary file 1 [file appendix_main.tex]

\documentclass{article}

% if you need to pass options to natbib, use, e.g.:
%     \PassOptionsToPackage{numbers, compress}{natbib}
% before loading neurips_2020

% ready for submission
% \usepackage{neurips_2020}

% to compile a preprint version, e.g., for submission to arXiv, add add the
% [preprint] option:
%     \usepackage[preprint]{neurips_2020}

% to compile a camera-ready version, add the [final] option, e.g.:
%     \usepackage[final]{neurips_2020}

% to avoid loading the natbib package, add option nonatbib:
%  \usepackage[nonatbib]{neurips_2020}
 \usepackage[final]{neurips_2020}

\usepackage[square,numbers]{natbib}
\bibliographystyle{abbrvnat}
\input{macros.tex}

\title{Supplementary Information for ``Regularizing Towards Permutation Invariance in Recurrent Models''}
% \title{Regularizing Towards Permutation Invariance in Recurrent Models}

% The \author macro works with any number of authors. There are two commands
% used to separate the names and addresses of multiple authors: \And and \AND.
%
% Using \And between authors leaves it to LaTeX to determine where to break the
% lines. Using \AND forces a line break at that point. So, if LaTeX puts 3 of 4
% authors names on the first line, and the last on the second line, try using
% \AND instead of \And before the third author name.

\author{%
  Edo Cohen-Karlik \\
  Tel Aviv University, Israel\\
  \texttt{edocohen@mail.tau.ac.il} \\
  % examples of more authors
   \And
   Avichai Ben David \\
  Tel Aviv University, Israel\\
  \texttt{avichaib@mail.tau.ac.il} \\
   \AND
   Amir Globerson\\
   Tel Aviv University, Israel\\
   and Google Research\\
   \texttt{gamir@post.tau.ac.il}\\
  % \And
  % Coauthor \\
  % Affiliation \\
  % Address \\
  % \texttt{email} \\
  % \And
  % Coauthor \\
  % Affiliation \\
  % Address \\
  % \texttt{email} \\
}

\begin{document}

\maketitle

% \begin{abstract}
% \input{abstract.tex}
% \end{abstract}

% \input{introduction.tex}

% \input{formulation.tex}

% \input{rnns_for_parity}

% \input{regularization.tex}

% \input{related_work.tex}

% \input{experiments.tex}

% \input{discussion.tex}

% \section{Broader Impact}
% In this work, we analyze an approach for learning recurrent models in cases where there is an underlying permutation invariance. The method can improve sequence labeling systems. We do not see any ethical aspects with the contribution. Societal aspects are positive in terms of improving accuracy of models in healthcare for example.

% % \nocite{ruiz2019invariance,sokolic2016generalization, jakubovitz2019generalization}
% \nocite{*}
% \bibliography{bib}

% \pagebreak

\appendix
\input{appendix_a}
\input{appendix_b}
\input{appendix_c}
\bibliography{bib}
\end{document}
